# Supplementary material for: Suppression of wall modes in rapidly rotating Rayleigh-B\'enard convection by narrow horizontal fins
Source: arXiv:2304.01136 source file (2023-04-03)
Supplement: Supplementary file 1 [file Supplemental_material.pdf]

# Supplemental material
# How to suppress wall modes
# in rapidly-rotating Rayleigh-Bénard convection

Louise Terrien* and Benjamin Favier†

*Aix Marseille Univ, CNRS, Centrale Marseille, IRPHE, Marseille, France*

Edgar Knobloch‡

*Department of Physics, University of California*

*at Berkeley, Berkeley, California 94720, USA*

(Dated: April 3, 2023)

## I. SIMULATIONS PARAMETERS

For each simulation, we start by fixing the Ekman number $E$. The critical Rayleigh number for the appearance of wall modes is then obtained using the result of [1]:

$$Ra_c^{\text{wall}} = \pi^2\sqrt{6\sqrt{3}}E^{-1} + 46.49E^{-2/3} \tag{1}$$

which is the first order correction to the asymptotic results obtained in [2, 3].

The size of the domain in the periodic direction $y$ is related to the most unstable wave number predicted to be [1, 4]

$$k_y = \pi\sqrt{2+\sqrt{3}} - 34.97E^{1/3} \tag{2}$$

which is again an extension of the asymptotic result of [2, 3]. Most simulations are performed with two unstable wavelengths along the $y$ direction, i.e. with $L_y = 4\pi/k_y$. For some cases, we have checked that increasing $L_y$ further leads to a relative error on the computed growth rate of at most 7%.

The domain size $L_x$ in the $x$ direction is chosen to minimize interactions between the two wall modes traveling (in opposite directions) along the boundaries. We use the scaling of the wall mode thickness obtained from linear stability analysis [2]:

$$\delta_0 = E^{1/3} \ . \tag{3}$$

For most simulations, the shortest distance between the two vertical walls is chosen to be $20\delta_0$ thus providing sufficient scale separation between the two vertical walls for each wall mode to be independent. We have checked that this is indeed the case by reducing this distance to $10\delta_0$ without noticeable modifications to our results. When we include barriers of width $\epsilon$, the domain size is increased in the $x$ direction according to $L_x = 20\delta_0 + 2\epsilon$ so that the shortest distance between the two barriers is always $20\delta_0$ irrespective of the barrier width.

The critical Rayleigh number for bulk convection is estimated from [5]:

$$Ra_c^{\text{bulk}} = \left(3(\pi^2/2)^{2/3} - 9.63E^{1/6}\right)E^{-4/3} \ . \tag{4}$$


* louise.terrien@ens-paris-saclay.fr
† benjamin.favier@cnrs.fr
‡ knobloch@berkeley.edu

| $E$ | $Ra_c^{\text{wall}}$ | $Ra_c^{\text{bulk}}$ | $Ra$ | $k_y$ | $\delta_0$ | $L_x$ | $L_y$ | $\mathcal{E}$ | $\mathcal{N}$ |
|---|---|---|---|---|---|---|---|---|---|
| $10^{-4}$ | $3.40 \times 10^5$ | $1.43 \times 10^6$ | $6.80 \times 10^5$ | 4.45 | 0.046 | 0.93 | 2.83 | [2120-2560] | 11 |
| $3 \times 10^{-5}$ | $1.11 \times 10^6$ | $7.51 \times 10^6$ | $2.22 \times 10^6$ | 4.98 | 0.031 | 0.62 | 2.52 | 2980 | 11 |
| $10^{-5}$ | $3.28 \times 10^6$ | $3.38 \times 10^7$ | $6.56 \times 10^6$ | 5.32 | 0.022 | 0.43 | 2.36 | 3480 | 11 |
| $3 \times 10^{-6}$ | $1.08 \times 10^7$ | $1.74 \times 10^8$ | $2.17 \times 10^7$ | 5.56 | 0.014 | 0.29 | 2.26 | 4160 | 11 |
| $10^{-6}$ | $3.23 \times 10^7$ | $7.73 \times 10^8$ | $6.46 \times 10^7$ | 5.72 | 0.01 | 0.2 | 2.20 | 4820 | 11 |
| | | | $3.1 \times 10^9$ | | | 0.3 | 1.10 | [11264:17280] | 13 |

TABLE I. List of numerical parameters for all simulations described in this paper. The critical Rayleigh number of wall modes, $Ra_c^{\text{wall}}$, is taken from [1] while that of bulk convection, $Ra_c^{\text{bulk}}$, is taken from [5]. The most unstable wave number along the homogeneous direction $k_y$ is taken from [1]; $\delta_0$ is the estimated width of the wall mode (see also [6]). $L_x$ is the size of the numerical domain transverse to the vertical walls and is taken to be $20\delta_0$. $L_y$ is the size of the numerical domain in the homogeneous direction and is taken to be $4\pi/k_y$. $\mathcal{E}$ is the number of hexahedral elements used to build the mesh. When a range of values is indicated, the smallest number of elements corresponds to the case without barrier while the largest corresponds to the case with barriers. $\mathcal{N}$ is the polynomial order used to discretize variables within elements. These values correspond to the cases without barriers.

For each case, we ensure that at least one element discretizes the horizontal Ekman layers of size $\sqrt{E}$. Along the vertical boundaries, we ensure that the first element is half the width of the wall mode, i.e. $\delta_0/2$. Numerical convergence is then tested by gradually increasing the polynomial order within each element.

Table I summarizes the simulation parameters for each Ekman number.

## II. INSULATING BARRIER WITH BAROCLINIC FLOWS

If the barrier is fully insulating (thus imposing $\nabla T \cdot \boldsymbol{n} = 0$ on all sides of the barrier where $\boldsymbol{n}$ is the local normal), there is no static equilibrium since isopycnals are not aligned with isotherms: a baroclinic flow invariant in the $y$ direction spontaneously develops. For the parameters considered here, this baroclinic flow eventually reaches a steady state so that instability to wall modes can be studied with respect to this new equilibrium state.

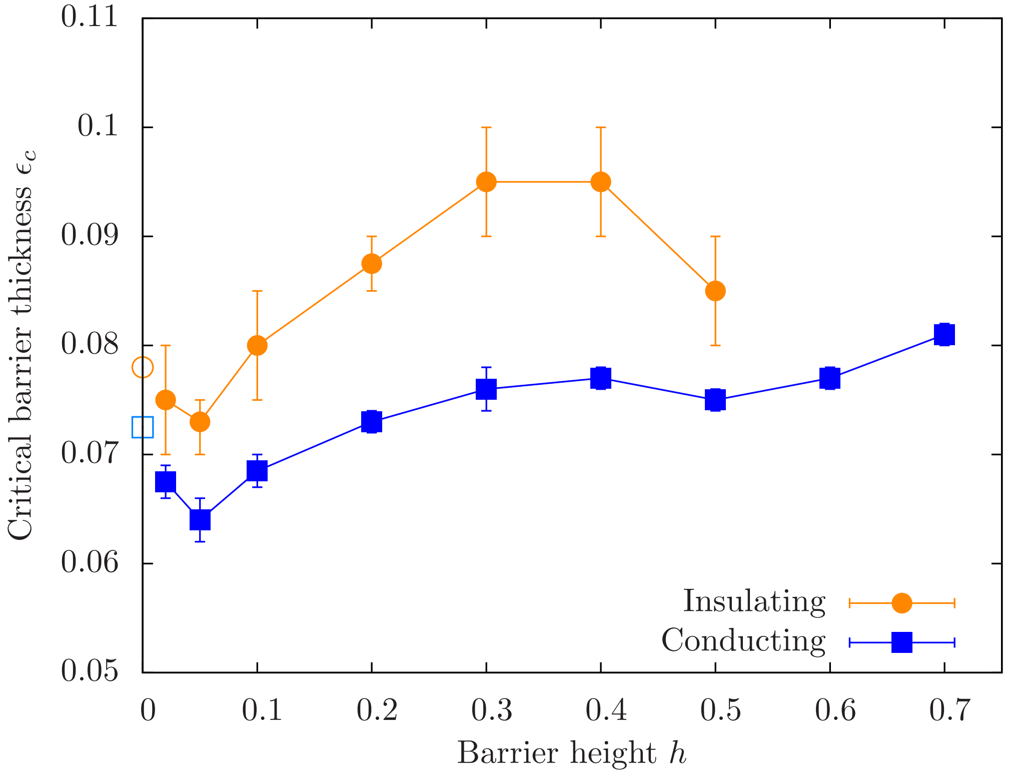


FIG. 1. Critical barrier width $\epsilon_c$ as a function of its height $h$ for $E = 10^{-4}$ and $Ra = 2Ra_c^{\text{wall}} \approx 6 \times 10^5$. The case of a conducting barrier (having the same diffusivity as that of the fluid) used in the main text is compared with the case of an insulating barrier (for which baroclinic flows develop). Empty symbols correspond to the case of an infinitely thin barrier.

To do so, we track the kinetic energy of perturbations around this baroclinic flow and vary the barrier width and height to find the critical parameters separating growing wall modes from decaying ones. The results are shown in Fig. 1 where we show the critical width $\epsilon$ for different heights for the parameters $E = 10^{-4}$, $Ra = 6 \times 10^5$ and $Pr = 1$. While the base state is now more complex, we observe that the barrier is still able to prevent the growth of wall modes. The critical curve is shifted to slightly larger widths, indicating the destabilizing nature of the baroclinic flow. Overall, these results confirm the relatively weak effect of the nature of the boundaries on the stability of wall modes even in the presence of an insulating barrier.

The influence of the boundary conditions applied on the barrier remains weak even in the turbulent regime. The results at $E = 10^{-6}$ and $Ra = 3 \times 10^9$ with 2 barriers discussed in the main text are nearly indistinguishable between conducting and insulating barriers.

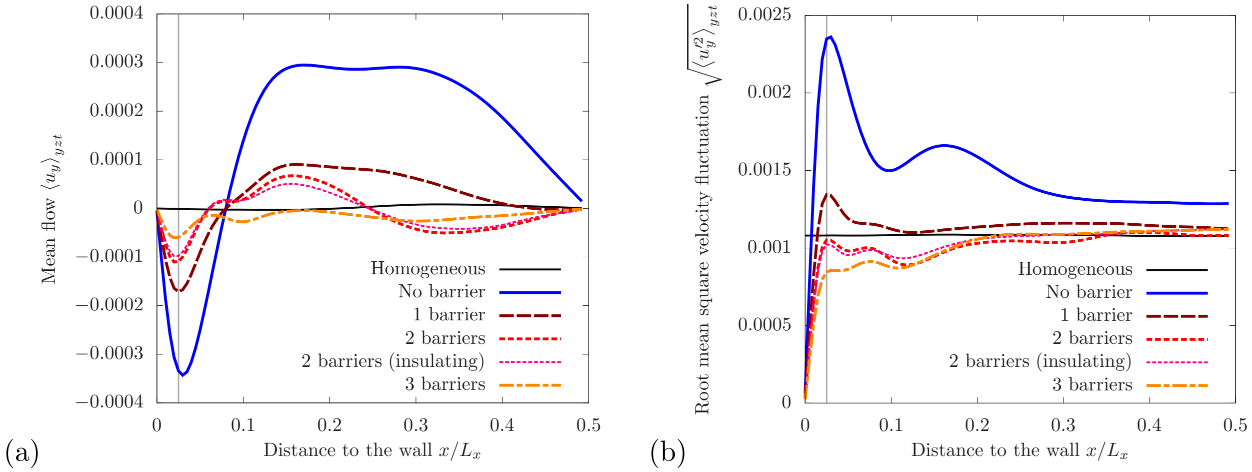


FIG. 2. Averaged hydrodynamical quantities as a function of the distance to the wall. (a) Mean flow in the homogeneous $y$ direction. (b) Rms of the velocity fluctuation $u'_y \equiv u_y - \langle u_y \rangle_{yzt}$ in the $y$ direction. Parameters are the same as those of Fig. 6 of the main text: $Ra = 3 \times 10^9$, $E = 10^{-6}$, $L_x = 0.3$, $L_y = 1.1$ and $Pr = 1$. The vertical grey line corresponds to the barrier width $\epsilon = 0.025$.

## III. DETAILS ON THE HYDRODYNAMICAL IMPACT OF THE BARRIERS

In this section, we show that in the presence of a suitable number of barriers we recover not only the heat flux profile of the homogeneous case but also the averages of various hydrodynamical quantities. In Fig. 2 we show averaged profiles of the zonal velocity and the rms fluctuations of the zonal velocity as a function of the distance to the wall. The average is performed over more than 500 free-fall times as in the main text as well as over $y$ and $z$. The zonal or mean flow parallel to the walls, $\langle u_y \rangle_{yzt}$, is a good indicator of whether wall modes have been significantly damped since it is zero by symmetry in the homogeneous case. Without barriers, we recover the so-called boundary zonal flows with a retrograde inner layer and a prograde outer layer [6–9]. While the first barrier is not sufficient to substantially reduce this flow, we find that only a residual mean flow persists once two or more barriers are introduced (Fig. 2(a)). We also confirm the similarity between conducting and insulating barriers for the particular case of two barriers.

Similar conclusions are obtained for fluctuating quantities as shown in Fig. 2(b) where we show the root-mean-square velocity in the $y$ direction. Apart from a small region close to the barrier, we recover the turbulence intensity of the homogeneous case once two or more

barriers are inserted.


[1] K. Zhang and X. Liao, The onset of convection in rotating circular cylinders with experimental boundary conditions, J. Fluid Mech. **622**, 63 (2009).

[2] J. Herrmann and F. H. Busse, Asymptotic theory of wall-localized convection in a rotating fluid layer, J. Fluid Mech. **255**, 183 (1993).

[3] E. Y. Kuo and M. C. Cross, Traveling-wave wall states in rotating Rayleigh-Bénard convection, Phys. Rev. E **47**, R2245 (1993).

[4] X. Liao, K. Zhang, and Y. Chang, On boundary-layer convection in a rotating fluid layer, J. Fluid Mech. **549**, 375 (2006).

[5] G. M. Homsy and J. L. Hudson, The asymptotic stability of a bounded rotating fluid heated from below: conductive basic state, J. Fluid Mech. **45**, 353 (1971).

[6] R. E. Ecke, X. Zhang, and O. Shishkina, Connecting wall modes and boundary zonal flows in rotating Rayleigh-Bénard convection, Phys. Rev. Fluids **7**, L011501 (2022).

[7] R. P. J. Kunnen, The geostrophic regime of rapidly rotating turbulent convection, J. Turb. **22**, 267 (2021).

[8] X. Zhang, R. E. Ecke, and O. Shishkina, Boundary zonal flows in rapidly rotating turbulent thermal convection, J. Fluid Mech. **915**, A62 (2021).

[9] B. Favier and E. Knobloch, Robust wall states in rapidly rotating Rayleigh–Bénard convection, J. Fluid Mech. **895**, R1 (2020).
